# Supplementary material for: Learning Depth Estimation for Transparent and Mirror Surfaces
Source: arXiv:2307.15052 source file (2023-07-27)
Supplement: Supplementary file 1 [file supplementary.pdf]

# Learning Depth Estimation for Transparent and Mirror Surfaces
# Supplementary material

Alex Costanzino* Pierluigi Zama Ramirez* Matteo Poggi*
Fabio Tosi Stefano Mattoccia Luigi Di Stefano
CVLAB, Department of Computer Science and Engineering (DISI)
University of Bologna, Italy
{alex.costanzino, pierluigi.zama, m.poggi, fabio.tosi5}@unibo.it

## 1. Additional Qualitative Results

**Virtual Depth Generation Alternatives.** We collect some additional samples to further motivate our aggregation strategy. Fig. 1 shows three examples from the Trans10k dataset, for which we report the RGB image and corresponding ground-truth segmentation mask, followed by depth maps predicted by DPT using the raw input, the in-painted image by using a constant, gray texture (N=1) or by aggregating the predictions obtained by picking 5 different colors to in-paint the masked image (N=5). We highlight how using a single texture makes some objects disappear in the predicted depth map, while this effect is neglected when exploiting multiple, different colors (rightmost column).

**Fine-Tuning Results on Trans10k and MSD.** We report additional qualitative results concerning monocular depth estimation networks fine-tuned according to our proposal. Fig. 2 shows some unseen examples of RGB images from Trans10k and MSD training sets, followed by corresponding depth maps predicted by DPT original weights, as well as by DPT after being fine-tuned on Trans10k and MSD testing set – respectively, by leveraging ground-truth segmentation masks or proxy segmentation masks predicted by Trans2Seg and MirrorNet. We can appreciate how, in both cases, the fine-tuning allows for the correction of errors made by the original DPT model, and the negligible differences between the two fine-tuned models.

**Ground-Truth vs Proxy Segmentation Masks.** In this section, we present additional examples concerning the use either of ground-truth segmentation mask or the predictions by Trans2Seg and MirrorNet within our pipeline. In Fig. 3, we collect some samples from Trans10k and MSD datasets – i.e., the same domain over which Trans2Seg and MirrorNet have been trained on. We can notice that using the two methods often produces similar results, but not always, as shown in the third row of Trans10k. This confirms that proxy segmentation masks are also effective for training purposes.

Fig. 4 shows, on the contrary, some examples from the Booster training dataset – i.e., a very different domain with respect to Trans10k and MSD datasets. In this case, we can observe how the segmentation masks produced by Trans2Seg and MirrorNet, sometimes, diverge significantly from the ground-truth annotations, e.g., as shown in the second row. This yields a virtual depth map that is completely different from the one we would expect, and supports the fact that our masking strategy is not suited for being used directly at test time. On the contrary, as we can observe in the rightmost column, by using ground-truth segmentation masks to obtain virtual depth maps and fine-tune a monocular network we obtain consistent results.

**Fine-tuned Monocular and Stereo Networks.** To conclude, Fig. 5 shows additional examples of predictions by the fine-tuned models, monocular (top) and stereo (bottom), on the Booster dataset. We can appreciate how the original models (*Base*) often fail in presence of ToM objects and surfaces, whereas after fine-tuning their depth is properly estimated. Furthermore, we highlight how this occurs both when using ground-truth segmentation masks – *Ft (GT mask)* – as well as when replacing these latter with the predictions by Trans2Seg and MirrorNet – *Ft (Proxy mask)*. Fig. 6 shows point clouds obtained from some of the samples reported in Fig. 5 – specifically, *Window* and *Oven* scenes, respectively in the second and seventh rows in Fig. 5. From these visualizations, we can better appreciate how the original monocular and stereo networks predict ToM surfaces that are not consistent with the real scene, while after fine-tuning they can reliably reconstruct the real geometry of the scene.

*These authors contributed equally to this work.

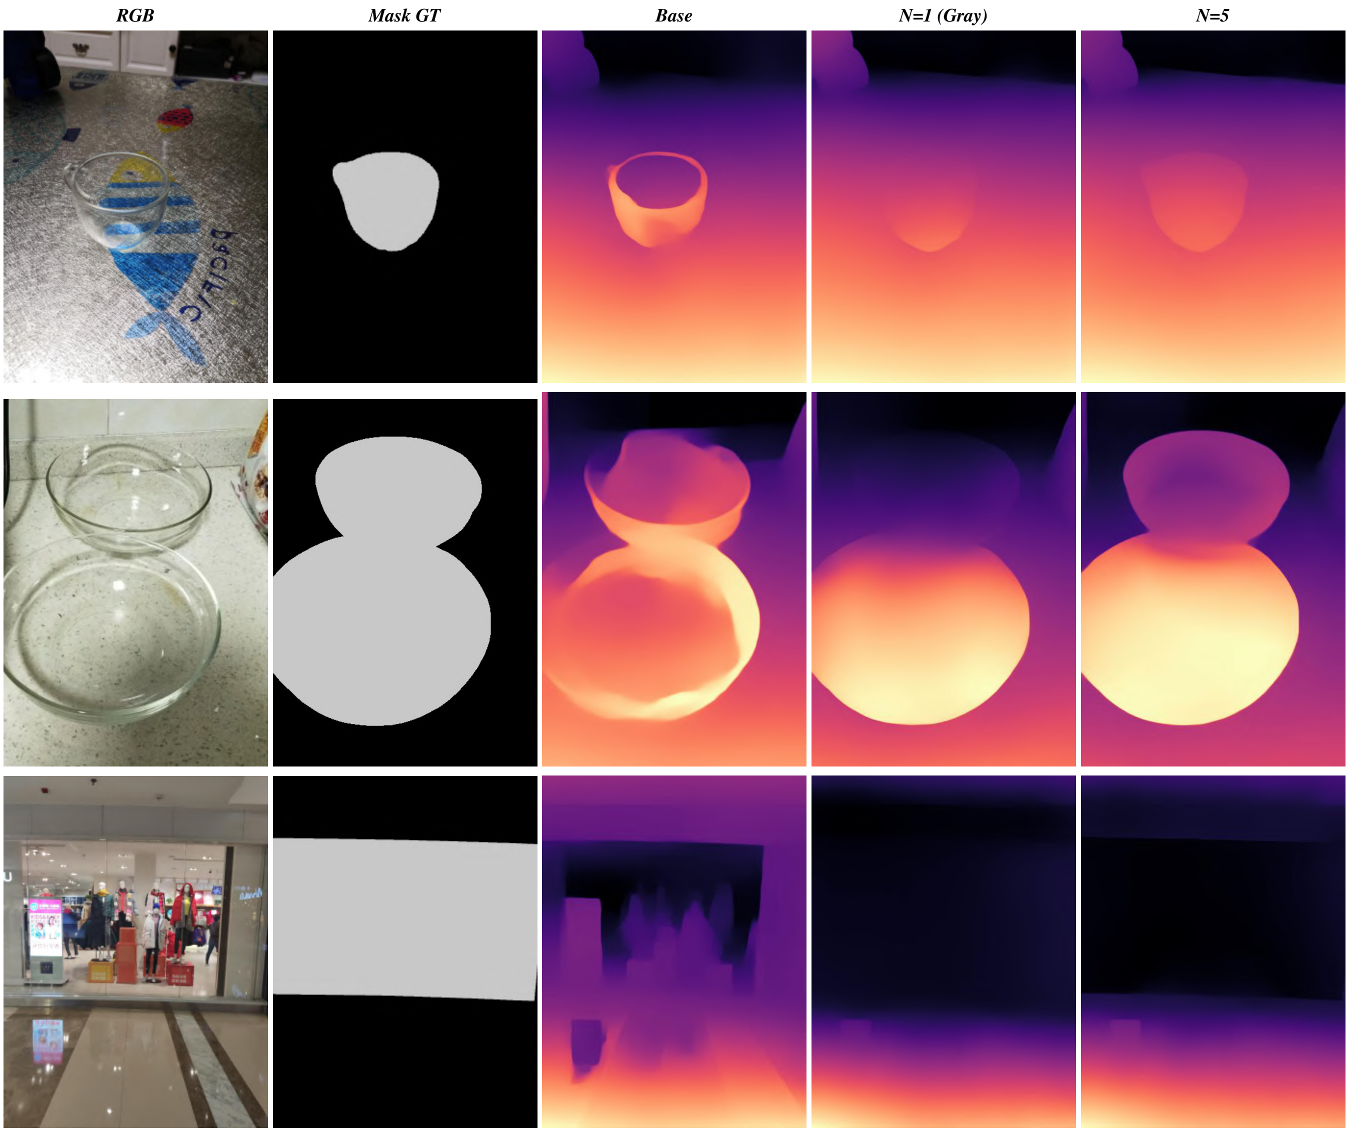


Figure 1. **Virtual Depth Generation Alternatives.** From left to right: RGB, ground-truth segmentation, DPT predictions on the RGB image, on the gray-masked input, and the median of five predictions on images masked with random colors.

**Handling of non-planar objects.** In Fig. 7 we show the point clouds of two scenes obtained by CREStereo (top) and DPT (bottom) under three different settings: with official weights (Base) on the RGBs, with official weights by in-painting inputs (Proxy Depth), and after fine-tuning with our technique on unaltered images. It shows that, in general, both in-painting and fine-tuning allow for recovering a better geometry than the Base version also for non-planar objects, with the fine-tuned networks achieving the most faithful reconstructions.

## 2. Additional Quantitative Results

**Performance on non-ToM surfaces** To prove the effectiveness of the fine-tuned models on scenes with only a few ToM surfaces, we tested the fine-tuned MiDaS and DPT (same network weights of Table 2, main paper - Ft. Virtual Depth row) on the NYU-V2 dataset [3], reporting the results in Table 1. We notice only negligible drops in performances – the strictest metric $\delta_{1.05}$ drops of less than 0.5%, which we consider a small price to pay for the large improvement on ToM surfaces. Indeed, in the Booster dataset (Table 2, main paper), $\delta_{1.05}$ for DPT Base vs FT-Virtual-Depth is improved by $\sim$17% on ToM objects.

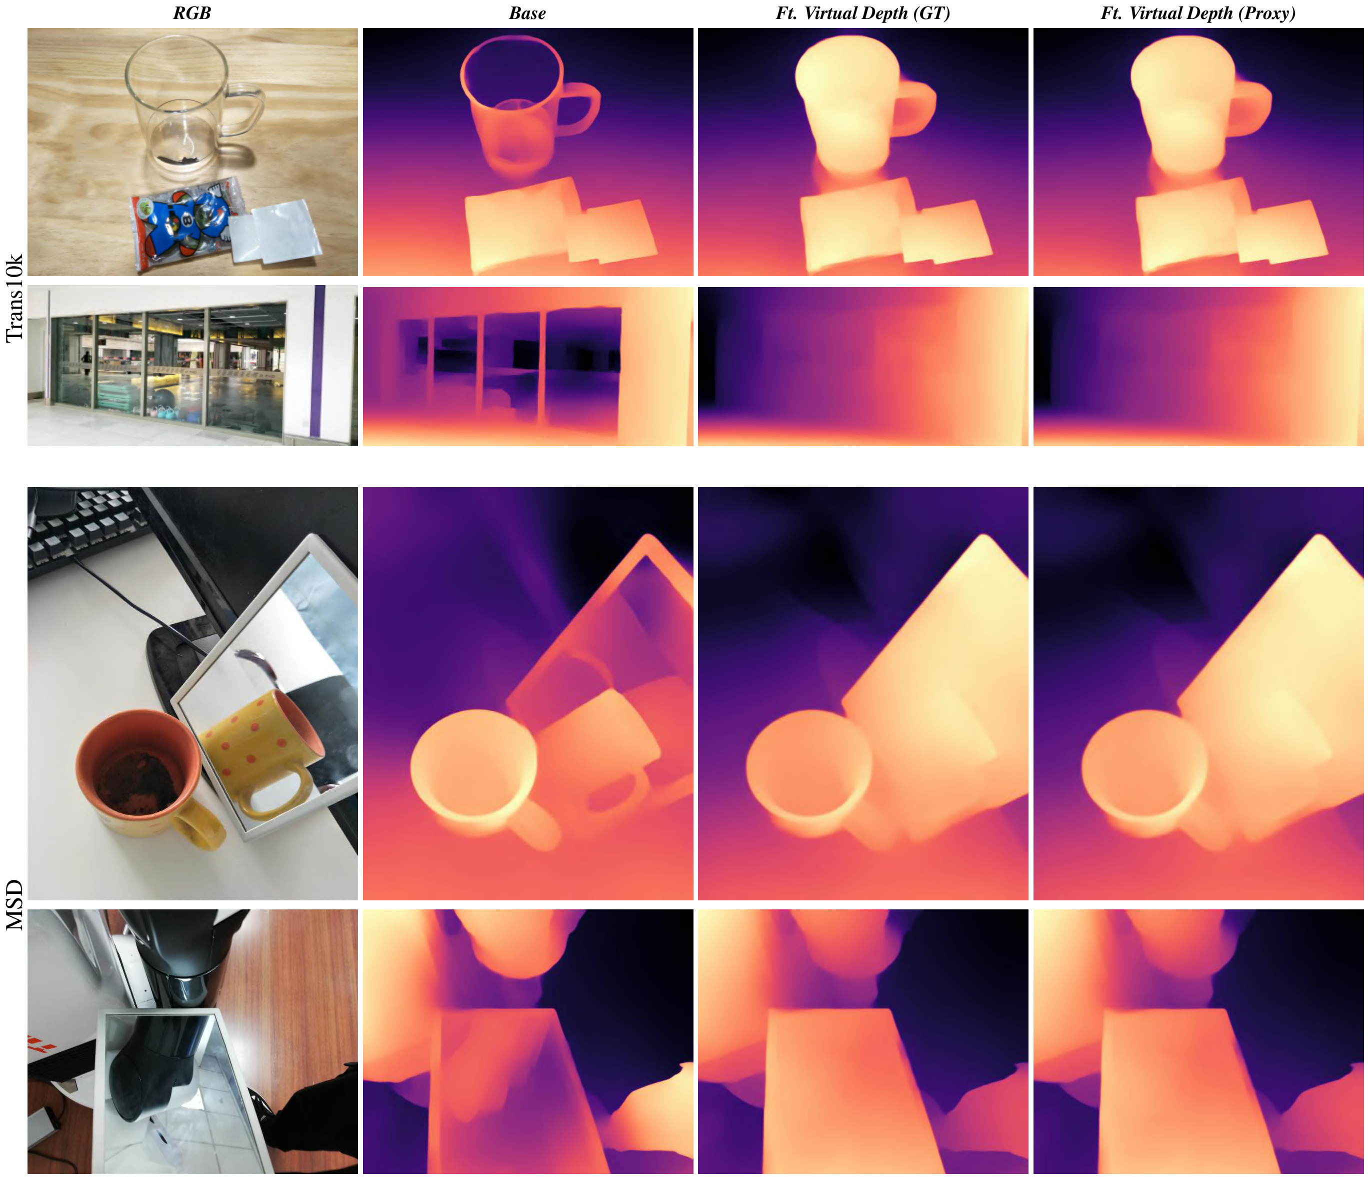


Figure 2. **Qualitative Results – DPT before and after fine-tuning.** From left to right: RGB, predictions by the original DPT weights and by two fine-tuned models, respectively using ground-truth segmentation masks or proxy segmentation masks predicted by Trans2Seg and MirrorNet. Model fine-tuned on test sets of Trans10k and MSD, tested on training sets of Trans10k and MSD.

| Category | Method | Model | $\delta < 1.25$ ↑ (%) | $\delta < 1.20$ ↑ (%) | $\delta < 1.15$ ↑ (%) | $\delta < 1.10$ ↑ (%) | $\delta < 1.05$ ↑ (%) | MAE ↓ (mm) | Abs. Rel ↓ | RMSE ↓ (mm) |
|---|---|---|---|---|---|---|---|---|---|---|
| All | Base | MiDaS | 91.68 | 87.13 | 79.17 | 64.77 | 39.04 | 27.17 | 0.09 | 40.16 |
| All | Ft. Virtual Depth | MiDaS | 90.38 | 85.89 | 77.97 | 63.74 | 38.57 | 29.40 | 0.09 | 44.37 |
| All | Base | DPT | 91.78 | 87.61 | 80.44 | 67.42 | 42.60 | 26.42 | 0.09 | 40.10 |
| All | Ft. Virtual Depth | DPT | 90.97 | 86.74 | 79.56 | 66.45 | 42.12 | 27.72 | 0.09 | 42.56 |

Table 1. **Mono results: Ft. Virtual Depth vs Base on NYU-V2.**

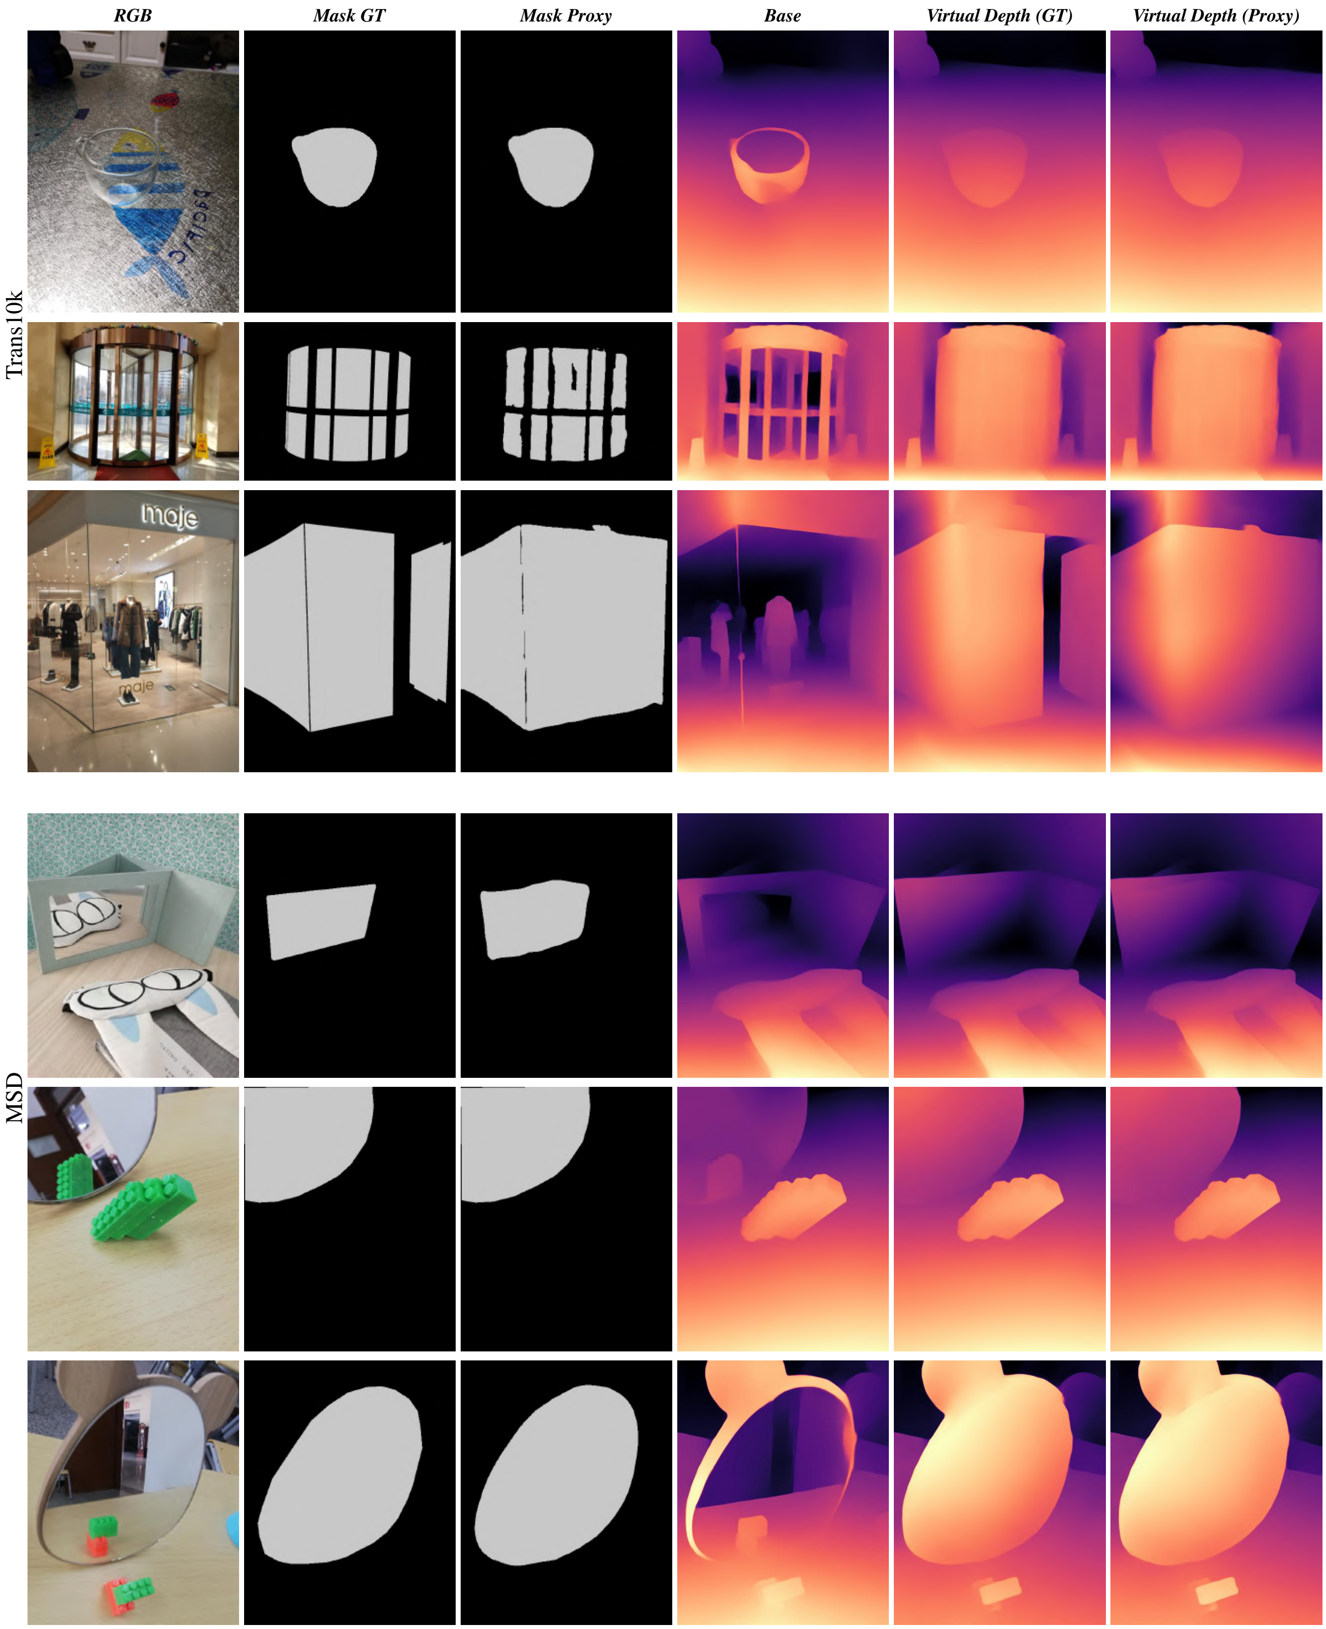


Figure 3. **Virtual Depth Qualitatives In-domain — GT vs Proxy.** From left to right: RGB, ground-truth and proxy segmentations, prediction with DPT on the RGB image, prediction with DPT on the median of five predictions by in-painting with either the ground-truth or semantic proxy masks on Trans10k and MSD.

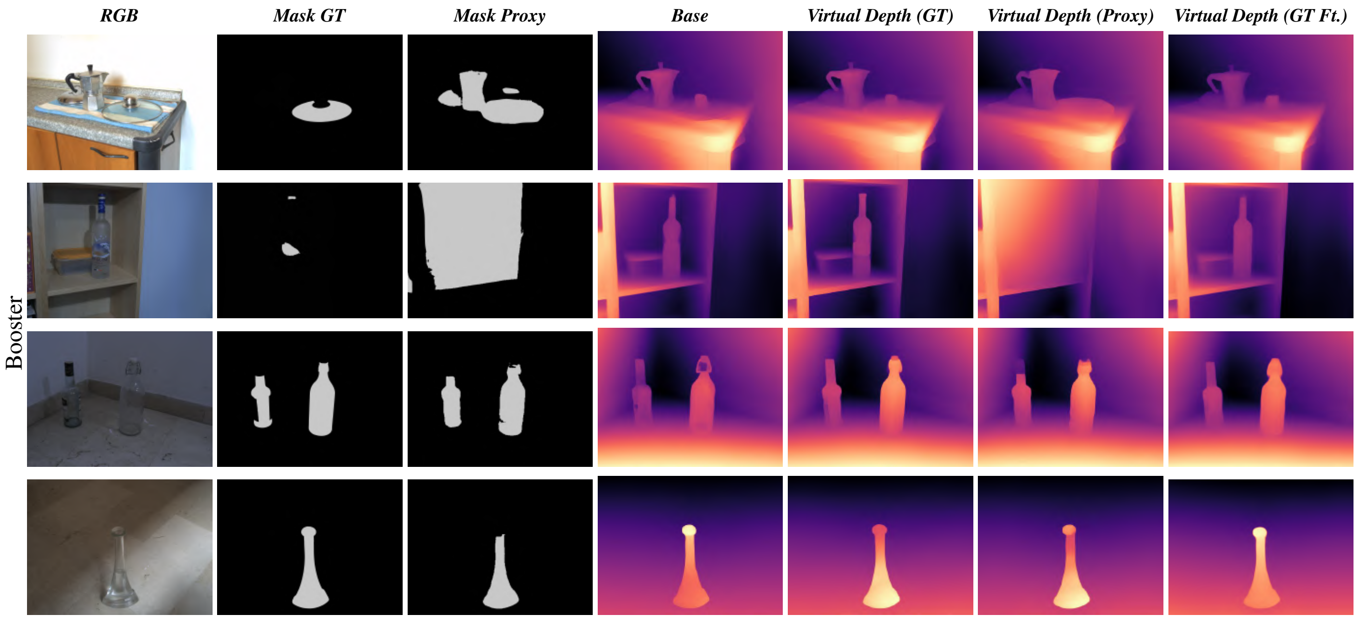


Figure 4. **Virtual Depth Qualitatives Out-of-domain: Booster – GT vs Proxy.** From left to right: RGB, ground-truth and proxy segmentations, prediction with DPT on the RGB image, prediction with DPT on the median of five predictions by in-painting with either the ground-truth or semantic proxy masks, prediction with DPT fine-tuned on Trans10k and MSD.

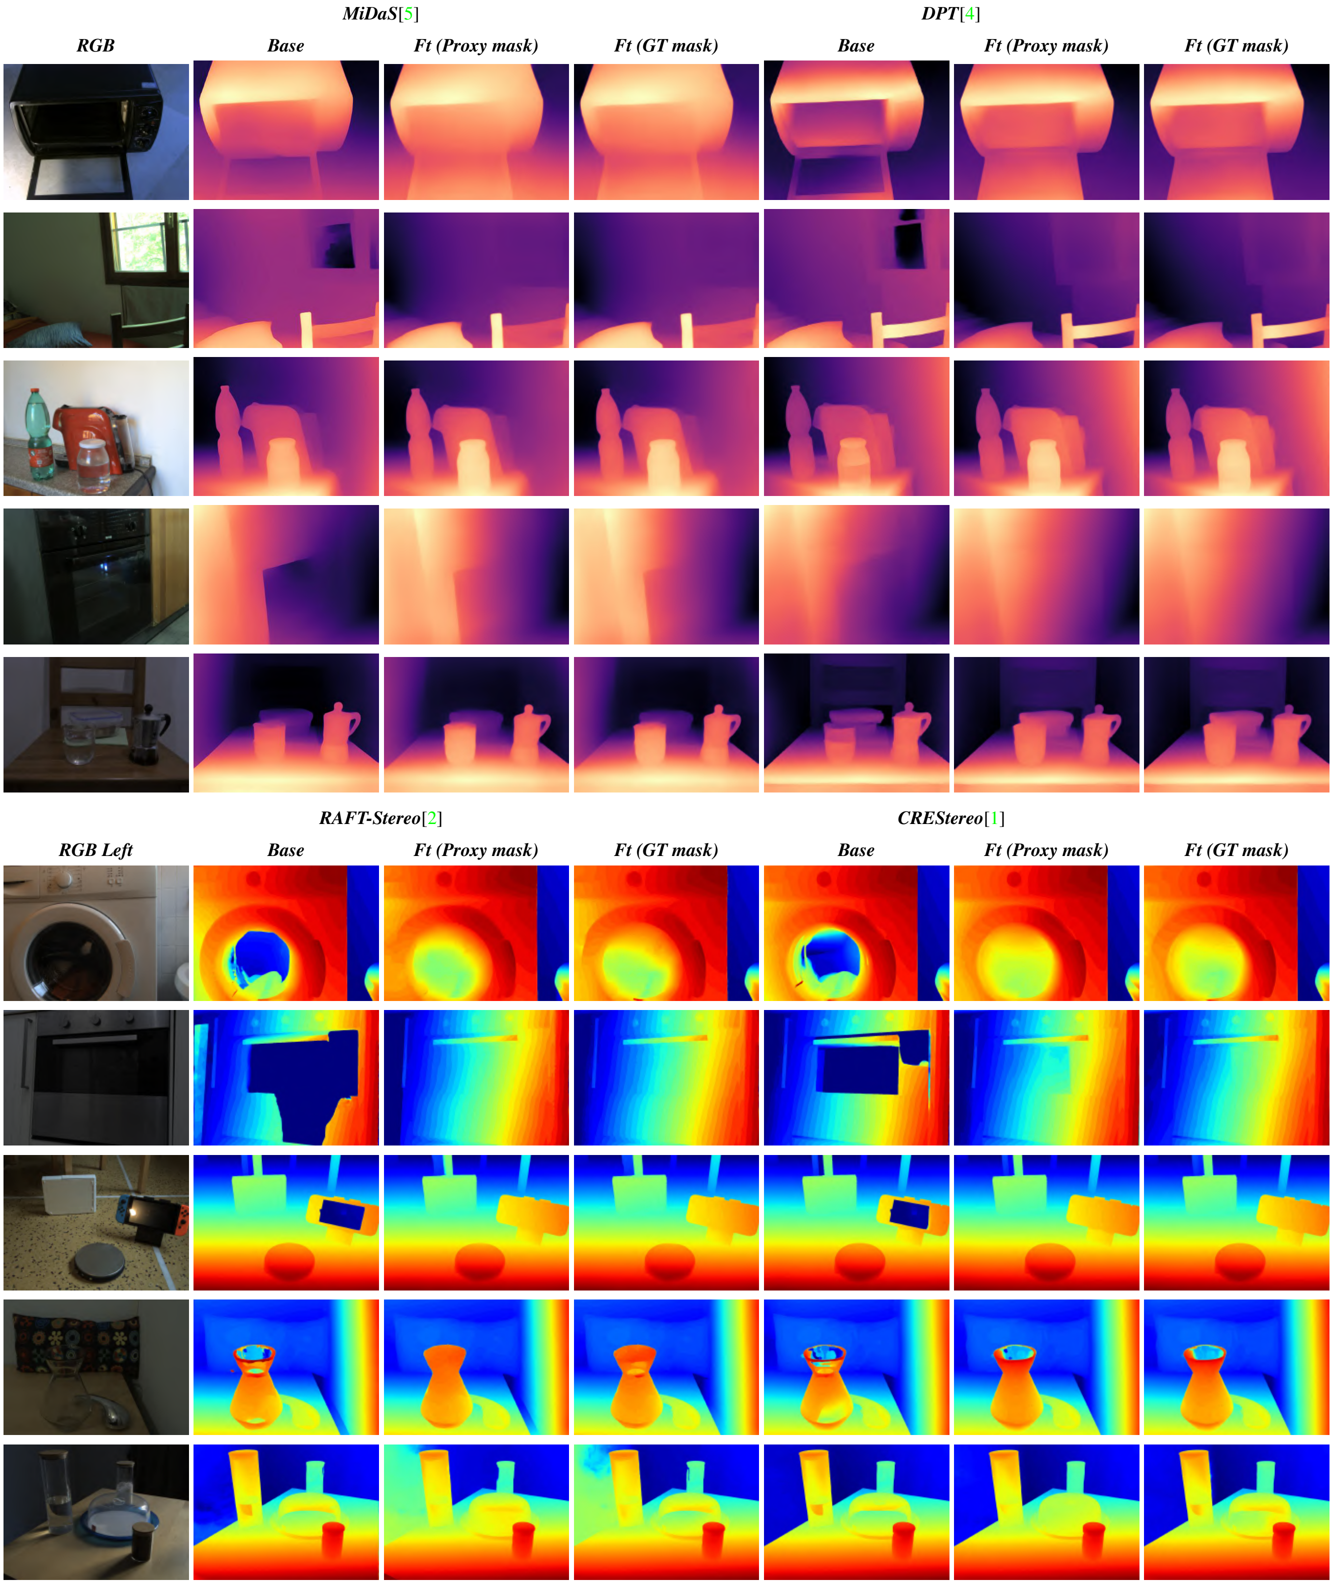


Figure 5. **Qualitative post fine-tuning results.** Examples of predictions by MiDaS and DPT (top), RAFT-Stereo and CREStereo (bottom). For each model, we show results achieved by the original model and by fine-tuned instances using proxy or GT segmentation masks.

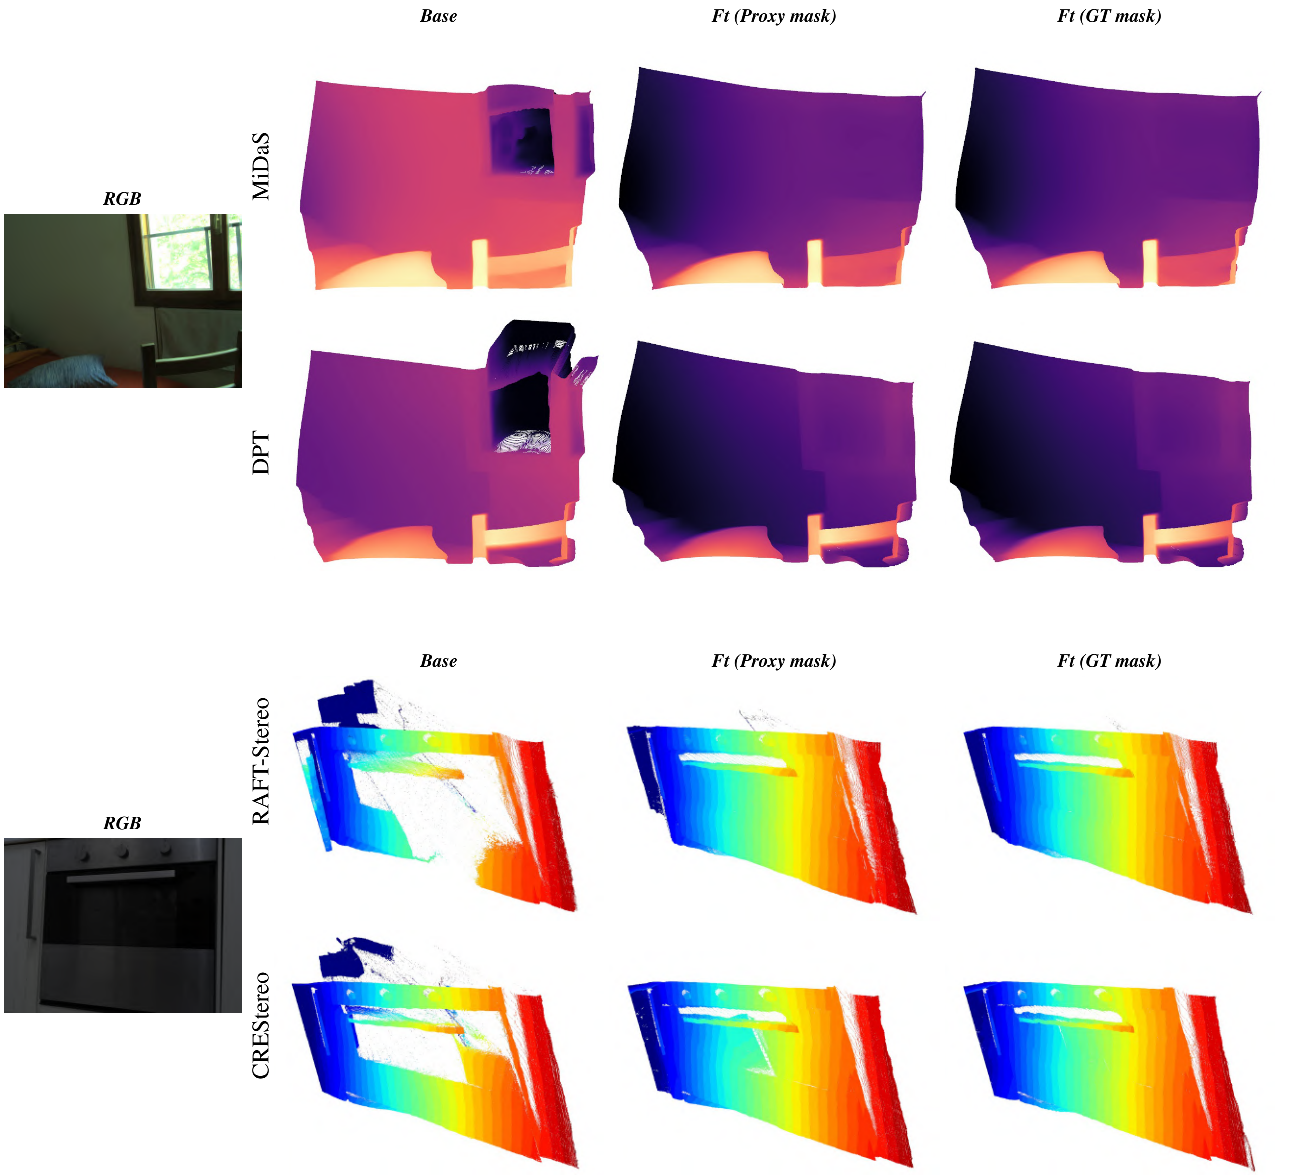


Figure 6. **Qualitative Point Cloud Post Fine-Tuning Results.** Examples of point cloud predictions by MiDaS and DPT (top), RAFT-Stereo and CREStereo (bottom). For each model, we show resulting point clouds achieved by the original model and by fine-tuned instances using proxy or GT segmentation masks.

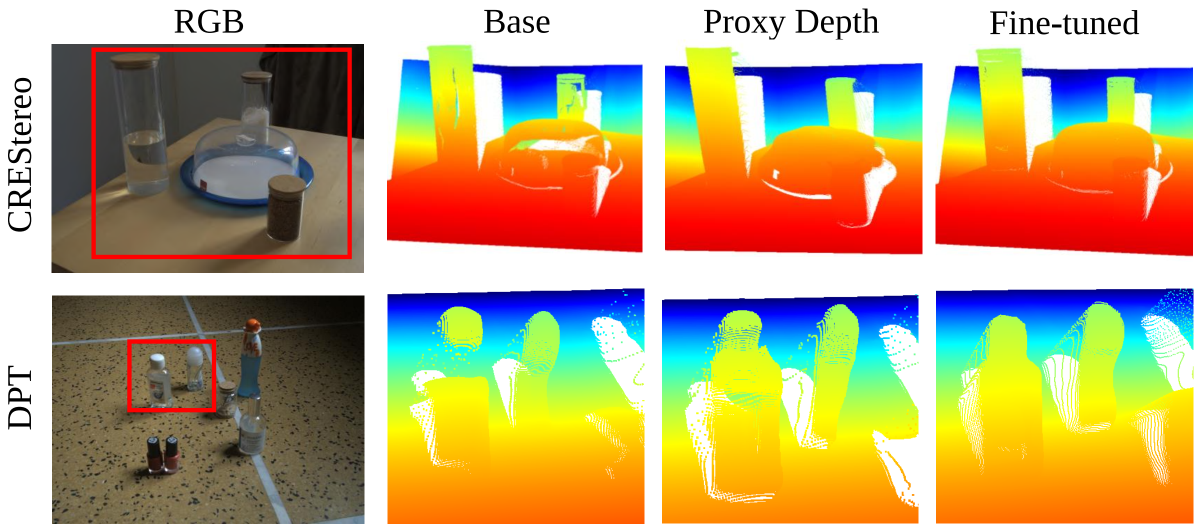

Figure 7. **Point Cloud Visualization.**

## References


[1] Jiankun Li, Peisen Wang, Pengfei Xiong, Tao Cai, Ziwei Yan, Lei Yang, Jiangyu Liu, Haoqiang Fan, and Shuaicheng Liu. Practical stereo matching via cascaded recurrent network with adaptive correlation. In *Proceedings of the IEEE/CVF Conference on Computer Vision and Pattern Recognition*, pages 16263–16272, 2022.

[2] Lahav Lipson, Zachary Teed, and Jia Deng. Raft-stereo: Multilevel recurrent field transforms for stereo matching. In *International Conference on 3D Vision (3DV)*, 2021.

[3] Pushmeet Kohli Nathan Silberman, Derek Hoiem and Rob Fergus. Indoor segmentation and support inference from rgbd images. In *ECCV*, 2012.

[4] René Ranftl, Alexey Bochkovskiy, and Vladlen Koltun. Vision transformers for dense prediction. *ICCV*, 2021.

[5] René Ranftl, Katrin Lasinger, David Hafner, Konrad Schindler, and Vladlen Koltun. Towards robust monocular depth estimation: Mixing datasets for zero-shot cross-dataset transfer. *IEEE Transactions on Pattern Analysis and Machine Intelligence*, 44(3), 2022.
